# Supplementary material for: Melting probe technology for subsurface exploration of extraterrestrial ice - Critical refreezing length and the role of gravity
Source: arXiv:1803.04883 source file (2018-03-13)
Supplement: Supplementary file 1 [file appendix.tex]

\section{Appendix: Derivation of the temperature field within the melt film}
The energy equation is
\begin{equation}
	u\frac{\partial T}{\partial r}+w\frac{\partial T}{\partial z}=\alpha_L\frac{\partial^2 T}{\partial z^2}
\end{equation}
On the left hand side we add the continuity equation, which must be zero due to incompressibility, multiplied by the temperature
\begin{equation}
	u\frac{\partial T}{\partial r}+w\frac{\partial T}{\partial z}+T\left( \frac{1}{r}\frac{\partial \left( r\,u \right)}{\partial r}+\frac{\partial w}{\partial z} \right)=\alpha_L\frac{\partial^2 T}{\partial z^2}
\end{equation}
The left hand side of equation ??? can now be rewritten by applying product rule, which can now be integrated with respect to $z$
\begin{equation}
	\int_{0}^{\delta}\left[\frac{1}{r}\frac{\partial \left(r\,u\,T\right)}{\partial r}+\frac{\partial \left(w\,T\right)}{\partial z}\right]dz=\alpha_L\int_{0}^{\delta}\frac{\partial^2 T}{\partial z^2}dz
\end{equation}
Applying Leibniz rule of integration yields
\begin{eqnarray}
	\frac{d}{rd r}\int_{0}^{\delta} r\,u\,T dz+w(r,\delta)\,T(r,\delta)-w(r,0)\,T(r,0)\nonumber\\
	=\alpha_L\left( \left. \frac{\partial T}{\partial z} \right|_{z=\delta}-\left. \frac{\partial T}{\partial z} \right|_{z=0} \right)
\end{eqnarray}
Substituting the boundary conditions into ??? yields
\begin{eqnarray}
\frac{d}{rd r}\int_{0}^{\delta} r\,u\,T dz -\frac{\rho_S}{\rho_L}W_0 T_m\nonumber\\
=\alpha_L\left( -\frac{\rho_SW_0}{k_L}h_m^*-\left. \frac{\partial T}{\partial z} \right|_{z=0} \right)
\end{eqnarray}
To simplify the solution of equation ???, the temperature profile is approximated by a quadratic polynomial in $z$-direction. The quadratic polynomial that satisfies the boundary conditions ??? is
\begin{eqnarray}
	T=T_w+z\left[ -\frac{2\left( T_H-T_m \right)}{\delta} +\frac{\rho_S W_0 h_m^*}{k_L}\right]\nonumber\\
	+z^2\left[ \frac{T_H-T_m}{\delta^2}-\frac{\rho_S W_0 h_m^*}{\delta\, k_L} \right]
\end{eqnarray}

\begin{eqnarray}
	\tilde{\delta}^2+\tilde{\delta}\frac{3\,\mathrm{Ste}+20}{2\tilde{W}_0}-\frac{10\,\mathrm{Ste}}{\tilde{W}_0^2}=0
\end{eqnarray}
The solution to equation ??? is
\begin{eqnarray}
	\tilde{\delta}=\frac{f(\mathrm{Ste})}{4\tilde{W}_0}
\end{eqnarray}
with
\begin{equation}
	f(\mathrm{Ste})=\sqrt{9\,\mathrm{Ste}^2+280\,\mathrm{Ste}+400}-3\,\mathrm{Ste}+20
\end{equation}
